# Supplementary material for: Calculation of intrinsic spin Hall conductivity by Wannier interpolation
Source: arXiv:1810.07637 source file (2018-10-17)
Supplement: Supplementary file 1 [file supp_mat.pdf]

# Supplemental Material: Calculation of intrinsic spin Hall conductivity by Wannier interpolation

Junfeng Qiao,<sup>1,2</sup> Jiaqi Zhou,<sup>1,2</sup> Zhe Yuan,<sup>3</sup> and Weisheng Zhao<sup>1,2,\*</sup>

<sup>1</sup>*Fert Beijing Institute, BDBC, Beihang University, Beijing 100191, China*

<sup>2</sup>*School of Electronic and Information Engineering,  
Beihang University, Beijing 100191, China*

<sup>3</sup>*The Center for Advanced Quantum Studies and Department of Physics,  
Beijing Normal University, 100875 Beijing, China*

(Dated: September 23, 2018)

## LIST OF FIGURES

|    |                                                                              |   |
|----|------------------------------------------------------------------------------|---|
| S1 | GaAs: <i>ab-initio</i> and Wannier interpolated band structure .....         | 2 |
| S2 | $\alpha$ -Ta: <i>ab-initio</i> and Wannier interpolated band structure ..... | 3 |
| S3 | $\alpha$ -Ta: k-resolved SHC in a slice of the BZ .....                      | 4 |
| S4 | $\beta$ -Ta: <i>ab-initio</i> and Wannier interpolated band structure .....  | 5 |
| S5 | $\beta$ -Ta: k-resolved SHC in a slice of the BZ .....                       | 6 |

---

\* weisheng.zhao@buaa.edu.cn

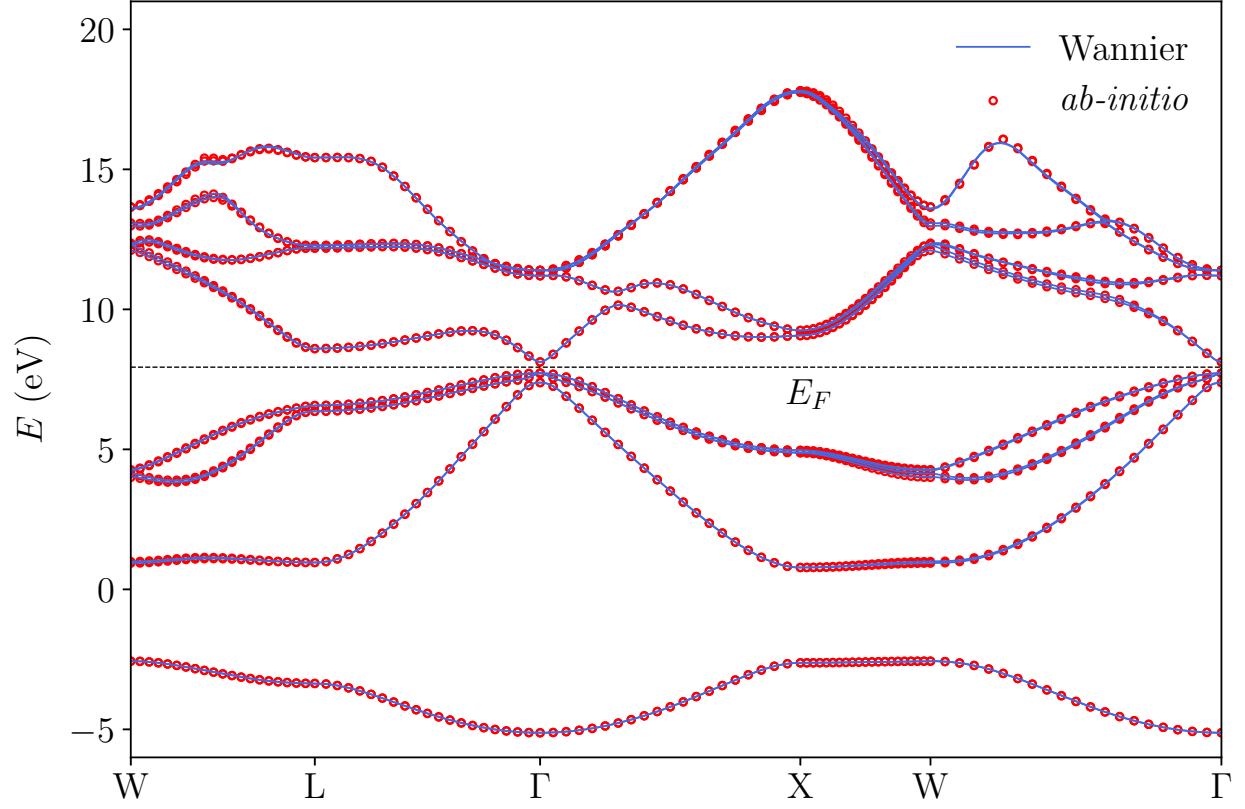

FIG. S1. Comparison of GaAs band structure obtained from *ab-initio* calculation (red circles) and the interpolated band structure by MLWFs (blue lines). The black dashed horizontal line corresponds to the Fermi energy. No disentanglement process is adopted. Scissors shift is not applied in the plot of band structure.

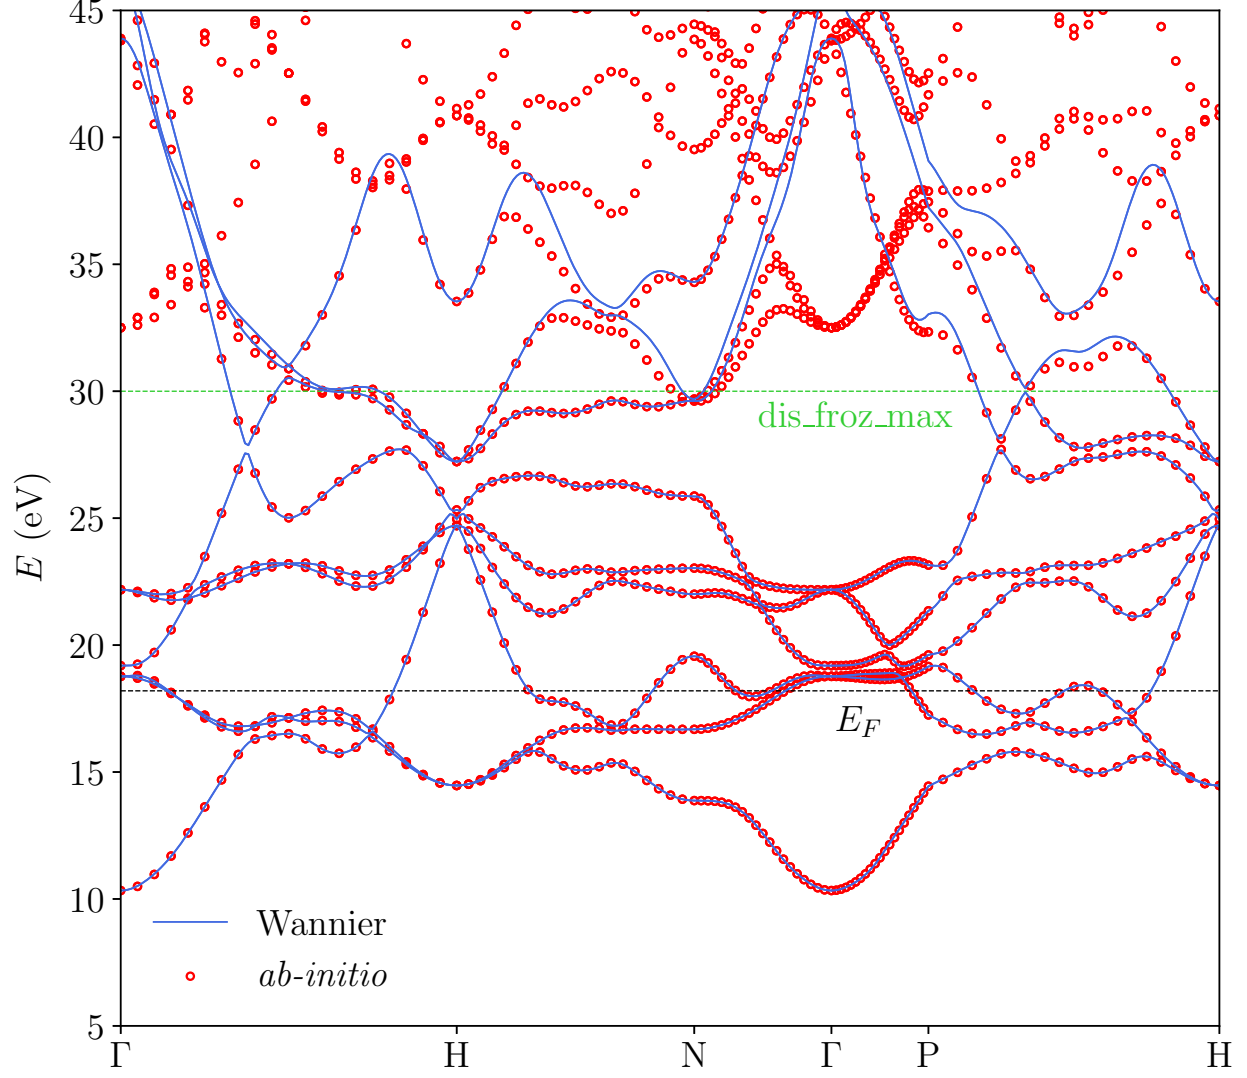

FIG. S2. Comparison of  $\alpha$ -Ta band structure obtained from *ab-initio* calculation (red circles) and the interpolated band structure by MLWFs (blue lines). The black dashed horizontal line corresponds to the Fermi energy, the green dashed horizontal line corresponds to the upper limit of the frozen inner window in the disentanglement process when constructing MLWFs.

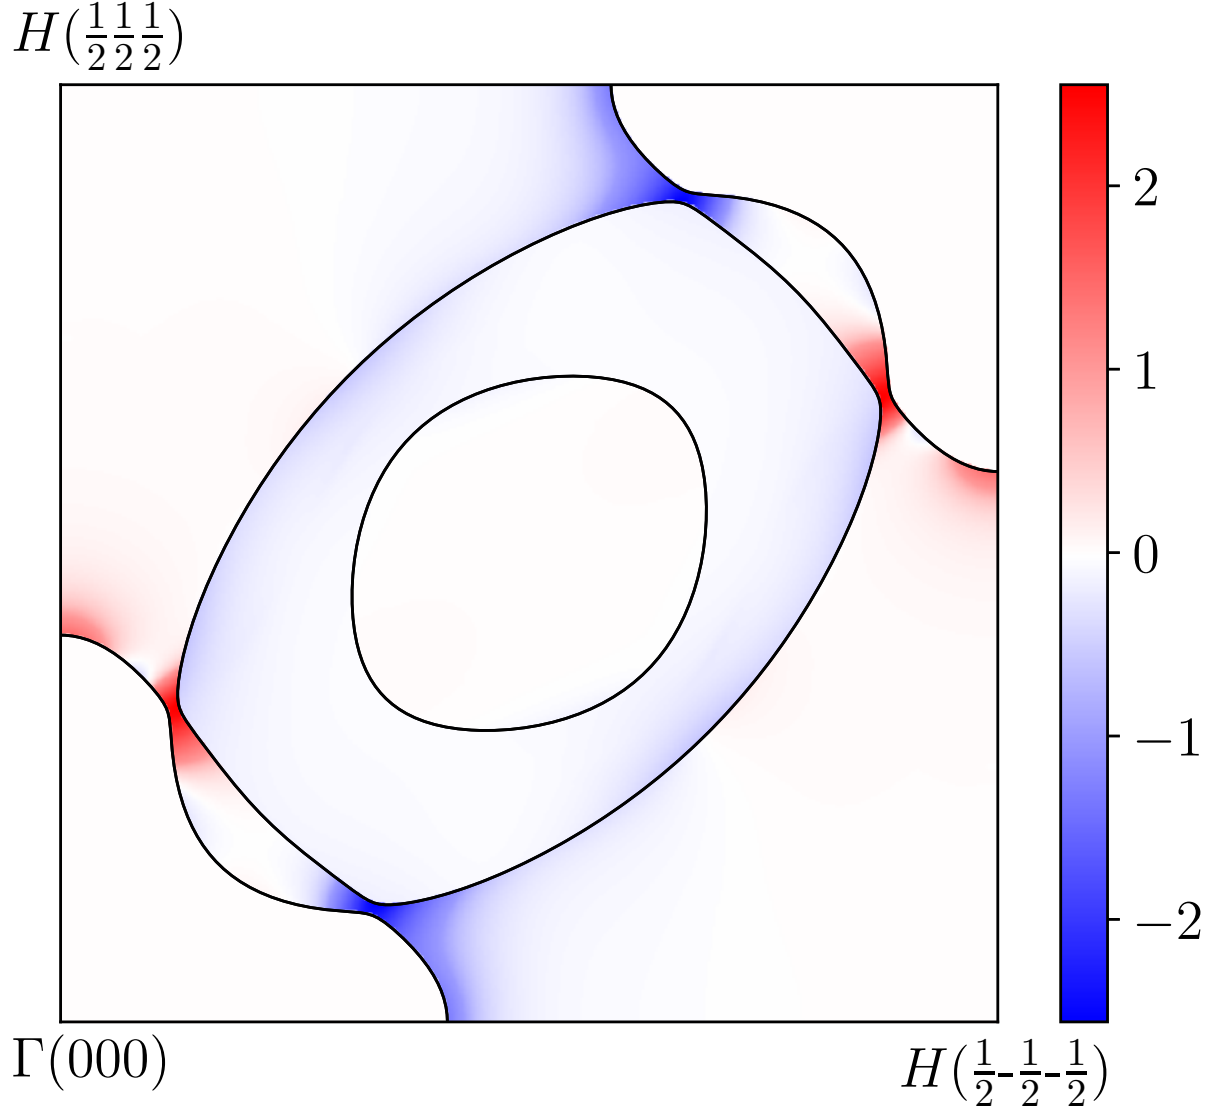

FIG. S3. SHC of  $\alpha$ -Ta in a slice of the BZ. The black lines are the intersection of the slice with the Fermi surface. The horizontal axis is the vector  $\vec{\Gamma\hat{H}} = (\frac{1}{2}, -\frac{1}{2}, -\frac{1}{2})$ , and the vertical axis is the vector  $\vec{\Gamma\hat{H}} = (\frac{1}{2}, \frac{1}{2}, \frac{1}{2})$ , which is normal to the horizontal axis. The color represents the logarithm [Equ.(51)] of Equ.(4) [in main text] without  $\mathbf{k}$  sum. The coordinates of the above mentioned vectors are fractional coordinates relative to the reciprocal lattice.

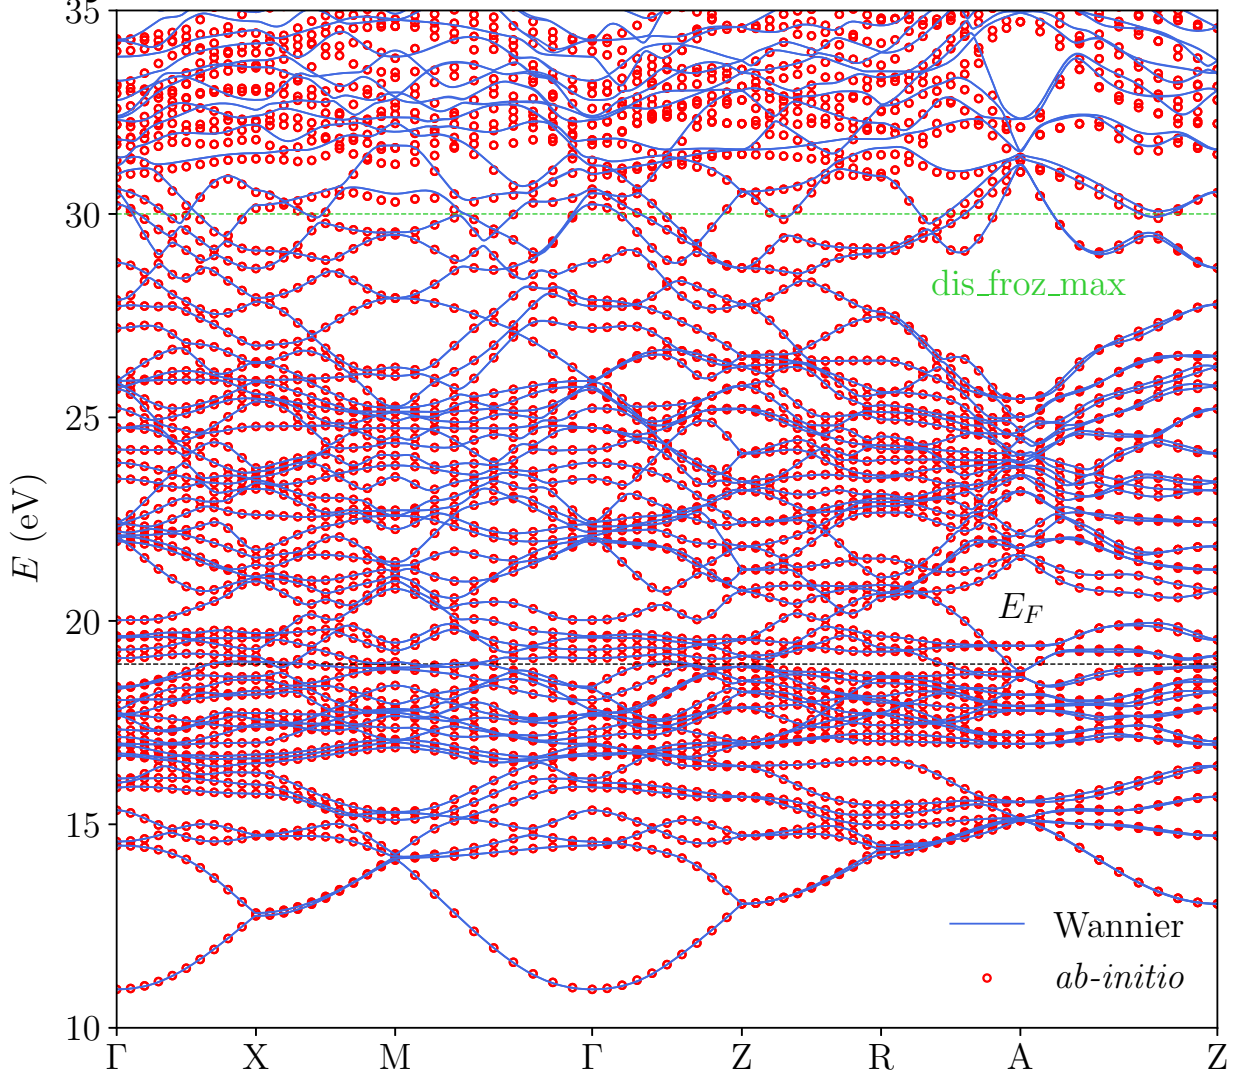

FIG. S4. Comparison of  $\beta$ -Ta band structure obtained from *ab-initio* calculation (red circles) and the interpolated band structure by MLWFs (blue lines). The black dashed horizontal line corresponds to the Fermi energy, the green dashed horizontal line corresponds to the upper limit of the frozen inner window in the disentanglement process when constructing MLWFs.

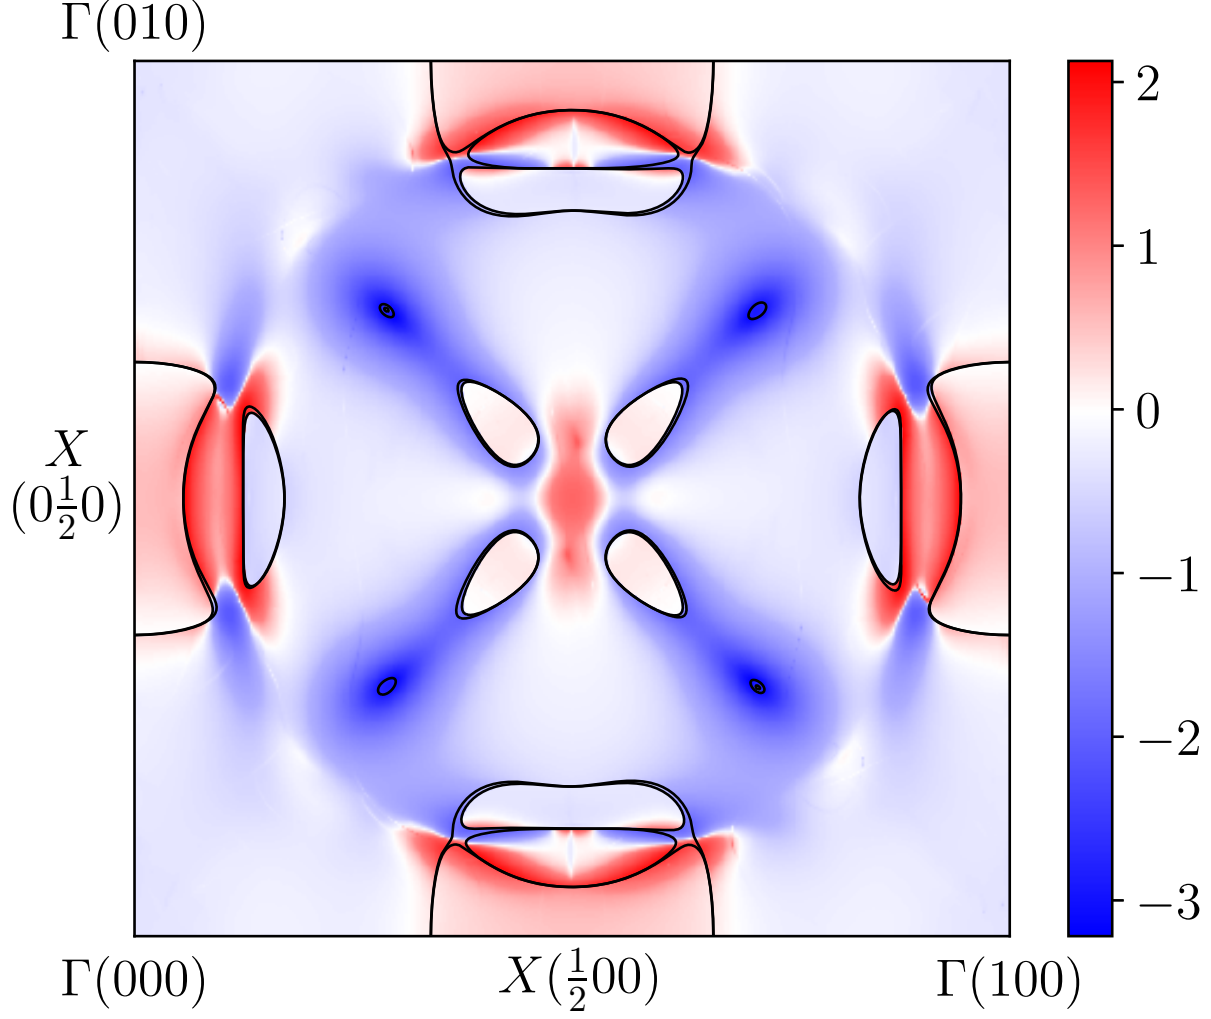

FIG. S5. SHC in a slice of the BZ. The slice is perpendicular to the reciprocal space  $\mathbf{c}$  axis. The black lines are the intersection of the slice with the Fermi surface. The horizontal axis is the vector  $2\vec{\Gamma X} = (1, 0, 0)$ , and the vertical axis is the vector  $2\vec{\Gamma X} = (0, 1, 0)$ , which is normal to the horizontal axis. The color represents the logarithm [Equ.(51)] of Equ.(4) [in main text] without  $\mathbf{k}$  sum. The coordinates of the above mentioned vectors are fractional coordinates relative to the reciprocal lattice.
